# Supplementary material for: Categorized Bandits
Source: arXiv:2005.01656 source file (2020-05-04)
Supplement: Supplementary file 1 [file MinMaxUCB.tex]

\documentclass[../main.tex]{subfiles}
 
\begin{document}

The lower bound stated in Theorem~\ref{th:lower_strong} seems to indicate that the best way to identify a suboptimal category is  by pulling its worst arm. Our second algorithm, whose pseudo-code is in Algorithm~\ref{algo:minmaxucb}, follows this idea. Let $\delta \in (0,1)$ be a confidence level. At each time step $t$, Algorithm~\ref{algo:minmaxucb} computes the best lower bound $C_m^+(t, \delta)$ and the worst upper bound $C_m^-(t, \delta)$ inside each category:
\begin{align*}
    C_m^+(t, \delta) &= \max_{k \in [K]} \widehat{\mu}_k^m(t) - \sqrt{\frac{2 \log\left( \frac{1}{\delta} \right)}{N_k^m(t)}} \\
    C_m^-(t, \delta) &= \min_{k \in [K]} \widehat{\mu}_k^m(t) + \sqrt{\frac{2 \log\left( \frac{1}{\delta} \right)}{N_k^m(t)}}
\end{align*}
Then it rejects suboptimal categories if their worst arm is statistically worse than the best arm of another category. Formally, let $\mathcal{A}(t, \delta)$ denote the set of active categories at time $t$ defined as follows:
\begin{equation*}
    \mathcal{A}(t, \delta) = \left\{ m \in [M] ; \forall n \ne m, C_n^+(t, \delta) \leq C_m^-(t, \delta) \right\}
\end{equation*}
As in the group-sparse case, they are three possible states

\noindent \textbf{i) $|\mathcal{A}(t, \delta)| = 0$:} no active  category;  pull all arms.

\noindent \textbf{ii) $|\mathcal{A}(t, \delta)| = 1$:}  one active category;   follow  \textsc{UCB}  on it.

\noindent \textbf{iii) $|\mathcal{A}(t, \delta)| > 1$:}  pull  all  arms of the active categories.

\begin{algorithm}[ht]
\SetAlgoLined
 Pull each arm once \\
 \While{$t \leq T$}{
  Compute $C_m^+(t, \delta)$ and $C_m^-(t, \delta)$ for all categories $m$ \\
  Compute $\mathcal{A}(t, \delta)$ the set of active categories\\
  \uIf{$|\mathcal{A}(t, \delta)| = 0$}{
    Pull all arms \\
  }
  \uElseIf{$|\mathcal{A}(t, \delta)| = 1$}{
    Let $C_t$ be the active category \\
    Pull arm $A_t \in \argmax_{k \in [K]} \widehat{\mu}^{C_t}_k(t) + \sqrt{\frac{2 \log\left(\frac{1}{\delta}\right)}{N^{C_t}_k(t)}}$ \\
  }
  \Else{
    Pull all arms in active categories \\
  }
 }
 \caption{\textsc{MinMaxUCB}($\delta$)} 
 \label{algo:minmaxucb}
\end{algorithm}

\begin{theorem}
With probability at least $1 - 2\delta MKT$, the regret of \textsc{MinMaxUCB}  is smaller than, with $\Delta_{\sharp,K} = \min_{m=2, \dots, M} \Delta_{m, K}$,
\begin{equation*}
    R_T \leq 8\sum_{k=2}^K   \max\left\{\frac{1}{\Delta_{1,k}}, \frac{4\Delta_{1,k}}{\Delta^2_{\sharp,K}}\right\}\log \frac{1}{\delta}  + \sum_{m=1}^M \sum_{K=1}^K \Delta_{m,k} + \sum_{m=2}^M \left( \frac{32 \log \frac{1}{\delta}}{(\Delta_{m, K})^2} \left( \sum_{k=1}^K \Delta_{m,k} \right) \right)
\end{equation*}
\label{th:upper_minmaxucb}
\end{theorem}

The first term of the regret corresponds to the UCB phase or the regret accumulated by the arms in the optimal category if it took too much time to rule out a sub-optimal one;  the second term corresponds to the regret incurred by arms in  suboptimal category, before it is eliminated. Choosing $\delta=1/2MKT^2$ (or even $\delta=T^{-3}$) gives a regret bound in expectation instead of with high probability.

\textsc{MinMaxUCB} outperforms, theoretically, \textsc{UCB} algorithm in this setting, since $\frac{\Delta_{m,k}}{\left( \Delta_{m,K} \right)^2} \leq \frac{1}{\Delta_{m,k}}$ because $\Delta_{m,k} \leq \Delta_{m,K}$, so the dependency in the gaps of arms in suboptimal categories is greatly reduced.

The major drawback of \textsc{MinMaxUCB} is that it only uses  the information of the best and worst arms of categories to discover suboptimal categories; it does not use the knowledge acquired by intermediate arms, which is used by the other algorithms we introduce in the following.
 
Notice that the algorithm \textsc{MinMaxUCB} consists in choosing $\mathbf{x}=(1,0,\ldots,0)$ and $\mathbf{y}=(0,\ldots,0,1)$ in \textsc{CatSE} instead of optimizing over their values. 
 
\subsection{Proof}

Let $\mathcal{E}$ be the good event defined by:
\begin{equation*}
    \mathcal{E} = \left\{  \forall m \in [M], \forall k \in [K], \forall u \in [T], \left|\widehat{\mu}_k^m - \mu_k^m\right| < \sqrt{\frac{2 \log \frac{1}{\delta}}{u}} \right\}
\end{equation*} 
Using the 1 sub-Gaussian hypothesis and a union bound, one obtains $\mathbb{P}(\mathcal{E}^c) \leq 2 \delta MKT$.

On $\mathcal{E}$, the optimal category is never eliminated. Otherwise, we would have:
\begin{equation*}
    \mu_1^m \geq \widehat{\mu}_1^m(t) - \sqrt{\frac{2 \log \frac{1}{\delta}}{N_1^m(t)}} > \widehat{\mu}_K^1(t) + \sqrt{\frac{2 \log \frac{1}{\delta}}{N_K^1(t)}} \geq \mu_K^1
\end{equation*}
which is impossible by assumption.

Now let us upper bound the number of times a sub-optimal category is active. By definition of the algorithm we have to upper bound the number of times we pull its worst arm. Let $t$ be the last time category $m$ is active. At time $t$, we have:
\begin{equation*}
    \widehat{\mu}_1^1(t) - \sqrt{\frac{2 \log \frac{1}{\delta}}{N_1^1(t)}} \leq \widehat{\mu}_K^m(t) + \sqrt{\frac{2 \log \frac{1}{\delta}}{N_K^m(t)}}
\end{equation*}
which implies
\begin{equation*}
    \Delta_{m, K} \leq 2 \left( \sqrt{\frac{2 \log \frac{1}{\delta}}{N_1^1(t)}} + \sqrt{\frac{2 \log \frac{1}{\delta}}{N_K^m(t)}} \right) = 4 \sqrt{\frac{2 \log \frac{1}{\delta}}{N_K^m(t)}}
\end{equation*}
where the last equality comes from the fact that $N_1^1(t) = N_K^m(t)$. Hence,
\begin{equation*}
    N_K^m(t) \leq \frac{32 \log \frac{1}{\delta}}{(\Delta_{m, K})^2}
\end{equation*}
The result follows with the classic proof of the UCB algorithm (Auer et al., 2002), the max term arising from the fact that the \textsc{UCB} algorithm pulls more times a suboptimal arm.
 
\end{document}
