# Supplementary material for: Categorized Bandits
Source: arXiv:2005.01656 source file (2020-05-04)
Supplement: Supplementary file 2 [file additional_experiments.tex]

\documentclass[../main.tex]{subfiles}
 
\begin{document}

In this section, we present numerical experiments illustrating the different perfomances of the algorithms we have introduced. We also compare them with two families of algorithms. The first one is algorithms for the multi-armed bandit framework, namely \textsc{UCB}~\cite{auer2002finite} and \textsc{Thompson Sampling}~\cite{thompson1933likelihood}; they are agnostic to the structure of the arms. The second family of algorithms is adapted to tree search, namely \textsc{UCT}~\cite{kocsis2006bandit}; they partially take into account the inherent structure. Specifically, they will just use the fact that  arms are grouped into categories but not necessarily that one category is optimal. 

We consider multiple scenarios for the different dominance hypothesis. In all experiments,  rewards are drawn from standard Gaussian distribution  and we report the average regret as a function of time, in a log-scale. \textsc{MinMaxUCB} and  \textsc{CatSE} were run with $\delta = \frac{1}{2MKT}$ and $\delta = \frac{1}{2MT}$, respectively. To implement \textsc{Thompson Sampling} and \textsc{Murphy Sampling}, we pulled each arm once and then sampled using a Gaussian prior. The simulations were ran until time horizon 100,000 and results were averaged over 500 independent runs.

\subsection{Group-sparse dominance}

Let us begin with the group-sparse dominance setting. An astute reader should have notice that the  SparseUCB algorithm~\cite{kwon2017sparse} cannot be used as the number of arms with positive expected reward is not known in advance in this setting. In this first scenario, we analyze a simple problem with two arms per category and two categories. Precisely, the expected rewards are 0.5 and 0 for the first category and 0 and 0 for the second category. The results are presented on Figure~\ref{fig:sparse1}.

\begin{figure}[ht]
\centering
\includegraphics[width=0.5\linewidth]{HSB_log_0_1.eps}
\caption{Regret of various algorithms as a function of time in the sparse dominance scenario.}
\label{fig:sparse1}
\end{figure}

As expected, \textsc{HSparseUCB} (implement here with the potential sampling improvement) outperforms \textsc{UCB} as it fully leverages the structure of the problem. Interestingly, \textsc{UCT} also outperforms \textsc{UCB} but it is still outmatched by \textsc{HSparseUCB}, with a striking difference in performances on this toy example.

\subsection{Strong dominance}

For the strong dominance assumption, we have  considered a simple scenario with two arms per category and two categories. More precisely, the expected rewards are 2 and 1 for the first category and 1 and 0 for the second category. The results are presented on Figure~\ref{fig:strong1}.

\begin{figure}[ht]
\centering
\includegraphics[width=0.5\linewidth]{HMAB_log_0_0.eps}
\caption{Regret of various algorithms as a function of time in the strong dominance scenario.}
\label{fig:strong1}
\end{figure}

Here again, the algorithms introduced outperform the baseline algorithms. \textsc{Murphy Sampling} seems to have the better guarantees, even if asymptotically, it has the same slope as \textsc{MinMaxUCB} and \textsc{CatSE}; the difference is mostly due to their exploration phase. Note also that \textsc{CatSE} performs slightly better than \textsc{MinMaxUCB} as a result of a better aggregation of the information.  

\subsection{First-order dominance}

Finally, we consider the first-order dominance setting. In this scenario, we look upon a problem with two arms per category and two categories. Precisely, the expected rewards are 5 and 4 for the first category and 4.5 and 0 for the second category. The results are presented on Figure~\ref{fig:fosd1}.

\begin{figure}[ht]
\centering
\includegraphics[width=0.5\linewidth]{HMAB_log_1_4.eps}
\caption{Regret of various algorithms as a function of time in the first-order dominance scenario.}
\label{fig:fosd1}
\end{figure}

Once again, \textsc{MS} and \textsc{CatSE} outperform baseline algorithms and both appear to have the same slope asymptotically with a significant difference between their regret. It is interesting to observe that \textsc{UCT} performed badly; as noticed in~\cite{coquelin2007bandit}, the convergence can be very slow.

In this section, we reproduce the experiments of section 6.2 and 6.3 but this time we do not present the average regret but instead, the ratio between the average regret divided by the lower bound on the regret for a particular dominance. We aim at analyzing the optimality of the proposed algorithms as the general result remains the same.

\subsection{Strong dominance}

On Figure~\ref{fig:alt_strong}, we repeat the experiment of section 6.2. \textsc{Murphy Sampling} appears to be to asymptotically optimal and the convergence takes place rapidly. On the contrary, \textsc{CatSE} and \textsc{MinMaxUCB} are asymptotically optimal up to a multiplicative factor (more or less 2). We thus find again the result of (Garivier et al.,2016). 

\begin{figure}[ht]
\centering
\includegraphics[width=0.5\linewidth]{HMAB_alt_0_0.eps}
\caption{Average regret over the regret lower bound in the strong dominance setting}
\label{fig:alt_strong}
\end{figure}

\subsection{First-order dominance}

On Figure~\ref{fig:alt_fosd}, we repeat the experiment of section 6.3. \textsc{Murphy Sampling} appears to perform better than the asymptotic lower bound on the expected regret. This can happen as the lower bound is only valid asymptotically. Nonetheless, we find again the same multiplicative factor for \textsc{CatSE} and \textsc{MinMaxUCB} algorithms. 

\begin{figure}[ht]
\centering
\includegraphics[width=0.5\linewidth]{HMAB_alt_1_4.eps}
\caption{Average regret over the regret lower bound in the first-order dominance setting}
\label{fig:alt_fosd}
\end{figure}
 
\subsection{Another one} 
 
$[[5, 4, 4, 4, 4], [4.5, 3, 3, 3, 0], [4.5, 3, 3, 3, 0], [4.5, 3, 3, 3, 0], [4.5, 3, 3, 3, 0]]$

\begin{figure}[ht]
\centering
\includegraphics[width=0.5\linewidth]{figures/HMAB_log_1_91.eps}
\caption{Regret of various algorithms as a function of time in the first-order dominance scenario.}
\label{fig:fod1}
\end{figure} 
 
\end{document}
