# Supplementary material for: Categorized Bandits
Source: arXiv:2005.01656 source file (2020-05-04)
Supplement: Supplementary file 3 [file proofs_alt.tex]

\documentclass[../main.tex]{subfiles}
 
\begin{document}

\subsection{Alternative proof}

Let us consider the case $M=2$ categories. Let $t$ be the last time we did not invoke the stopping rule, i.e.\ that category $2$ is still active. By Equation~\eqref{eq:CatSE1}, we have
\begin{equation*}
    \forall\, \mathbf{x} \in \Delta(K), \langle \mathbf{x}, \widehat{\mu}^1_{\sigma^1_t}(t) - \widehat{\mu}^2_{\sigma^2_t}(t) \rangle \leq 2 \| \mathbf{x} \|_2 \beta(t, \delta) \,,
\end{equation*}
where $\widehat{\mu}^m_{\sigma^m_t}(t)$ denotes the vector $\widehat{\mu}^1(t)$ ordered in decreasing order. On the clean event defined previously, this yields
\begin{equation*}
    \forall\, \mathbf{x} \in \Delta(K), \langle \mathbf{x}, \mu^1_{\sigma^1_t}(t) - \mu^2_{\sigma^2_t}(t) \rangle \leq 4 \| \mathbf{x} \|_2 \beta(t, \delta) \,.
\end{equation*}
Decomposing $\langle \mathbf{x}, \mu^m_{\sigma^m_t}  \rangle$ into $\langle \mathbf{x}, \mu^m_{\sigma^m_t} - \mu^m \rangle + \langle \mathbf{x}, \mu^m \rangle$ gives
\begin{align*}
    \forall\, \mathbf{x} \in \Delta(K), \langle \mathbf{x}, \mu^1 - \mu^2 \rangle &\leq 4 \| \mathbf{x} \|_2 \beta(t, \delta) + \langle \mathbf{x}, \mu^1 - \mu^1_{\sigma^1_t} \rangle + \langle \mathbf{x}, \mu^2_{\sigma^2_t} - \mu^2 \rangle \\
    &\leq \| \mathbf{x} \|_2 \left( 4 \beta(t,\delta) + \| \mu^1 - \mu^1_{\sigma^1_t} \|_2 + \| \mu^2_{\sigma^2_t} - \mu^2 \|_2 \right) \,,
\end{align*}
where the last line comes from the Cauchy–Schwarz inequality. In particular, taking $\mathbf{x} = \frac{\mu^1 - \mu^2}{\| \mu^1 - \mu^2 \|_1}$ we obtain
\begin{equation*}
    \|\mu^1 - \mu^2\|_2 \leq 4 \beta(t,\delta) + \| \mu^1 - \mu^1_{\sigma^1_t} \|_2 + \| \mu^2_{\sigma^2_t} - \mu^2 \|_2 \,.
\end{equation*}
Now let $\varepsilon > 0$ to be defined later. Thanks to the round-robin sampling phase, there exists $T^m_\varepsilon \in \mathbb{N}^\star$ such that $\forall\, t \geq T^m_\varepsilon$, $\sigma^m_t(i) = j$ with $i \ne j$ implies $|\mu^m_i - \mu^m_j | < \varepsilon$. If $t$ is large enough, then the right hand side of the previous inequality is bounded as
\begin{equation*}
    \|\mu^1 - \mu^2\|_2 \leq 4 \beta(t,\delta) + 2 \sqrt{K} \varepsilon \,.
\end{equation*}
Finally, for $\varepsilon < \frac{\| \mu^1 - \mu^2 \|_2}{2 \sqrt{K}}$, we obtain
\begin{equation*}
    N^2(t) \leq \max\{T^1_\varepsilon, T^2_\varepsilon\} + 32 \left(\log\frac{1}{\delta} + K \log 2 \right) \frac{1}{\left( \| \mu^1 - \mu^2 \|_2 - 2 \sqrt{K}\varepsilon \right)^2} \,.
\end{equation*}

It remains to characterize $T^m_\varepsilon$ for all m. It is easy to see that 
\begin{equation*}
    \mathbb{E}[T^m_\varepsilon] \leq \max_{k=1, \ldots, K-1} \frac{4}{\left( \mu^m_k - \mu^m_{k-1} \right)^2} \mathbf{1}\left\{\mu^m_k - \mu^m_{k-1} \geq \varepsilon \right\} \,.
\end{equation*}

\end{document}
