# Supplementary material for: Categorized Bandits
Source: arXiv:2005.01656 source file (2020-05-04)
Supplement: Supplementary file 4 [file confidence_set.tex]

\documentclass[../main.tex]{subfiles}
 
\begin{document}

\begin{proposition}
With probability at least $1 - \delta$, the following holds uniformly overall all $ \mathbf{x} \in \mathbb{R}^K$,
\begin{equation*}
    \langle \mathbf{x}, \widehat{\mu}^m(p) - \mu^m \rangle \leq  \left\lVert \mathbf{x} \right\rVert_2  \sqrt{ \frac{2}{p} \left( K \log 2 + \log\frac{1}{\delta} \right)} \,.
\end{equation*}
\end{proposition}
Fix $x \in \mathbb{R}$ and $\delta \in (0,1)$ a confidence level. According to (Lattimore and Szepesv{\'a}ri, 2018), we have with probability at least $1 - \delta$,
\begin{equation*}
    \left\lVert \widehat{\mu}(t) - \mu \right\rVert_{V_t} \leq  \sqrt{2 \left( K \log 2 + \log \frac{1}{\delta} \right)} \,.
\end{equation*}

If an agent pulls each arm sequentially, we are in the fixed design setting. In this case, (assuming $t$ is a multiple of $K$), we have $V_t = N(t) \mathbf{I}_K$, i.e.\ it is a diagonal matrix and we conclude.
 
\end{document}
